# Supplementary material for: Bayesian Nonparametric Multivariate Spatial Mixture Mixed Effects Models with Application to American Community Survey Special Tabulations
Source: arXiv:2009.12351 ancillary file (2020-09-25)
Supplement: Supplementary file 1 [file ACSST-supp-arxiv.pdf]

# Supplementary Material for Bayesian Nonparametric Multivariate Spatial Mixture Mixed Effects Models with Application to American Community Survey Special Tabulations

Ryan Janicki[a], Andrew M. Raim[a], Scott H. Holan[bc], and Jerry Maples[a]

[a]Center for Statistical Research and Methodology, U.S. Census Bureau
[b]Department of Statistics, University of Missouri
[c]Office of the Associate Director for Research and Methodology, U.S. Census Bureau

2020-09-25

**Abstract**

The supplementary material contains additional details on model specifications, as well as derivations of the full conditional distributions needed for the Gibbs sampler for posterior inference, for both the multivariate spatial model, as well as the multivariate spatial mixture model, introduced in the main paper. In addition, computational details for efficient construction of the multivariate spatial basis functions and the precision matrix of the latent Gaussian process are provided. Also, additional information about the variance estimates of the log-transformed direct estimates used in the numerical examples is given.

## A Introduction

Throughout, for notational convenience, let $i = 1, \ldots, n$ index both the areal units, $A \in \mathcal{D}$, and the variables within an area, $l = 1, \ldots, L$. Also, we use bracket notation, $[\boldsymbol{x} \mid \boldsymbol{y}]$, to denote a general conditional probability density of $\boldsymbol{x}$ given $\boldsymbol{y}$.

## B Gibbs Sampler for the Multivariate Spatial Model

The multivariate spatial model (MSM) can be written hierarchically, using the standard data, process, and parameter model formulation, which is popular in the spatial statistics literature. The data model is given by

$$Z_i = Y_i + \varepsilon_i,$$

where $Z_i$ are the direct survey estimates, $Y_i$ are the true values, and $\varepsilon_i \overset{\text{ind.}}{\sim} \mathrm{N}(0, D_i)$ for known sampling variances $D_i$. The process model is given by

$$Y_i = \boldsymbol{x}_i^\top \boldsymbol{\beta} + \boldsymbol{s}_i^\top \boldsymbol{\eta}$$
$$\boldsymbol{\eta} \sim \mathrm{N}_r\left(\mathbf{0}, \sigma_\eta^2 \boldsymbol{K}\right),$$

and the parameter model is

$$\boldsymbol{\beta} \sim \mathrm{N}_p\left(\mathbf{0}, \sigma^2_{\boldsymbol{\beta}} \boldsymbol{I}_{p\times p}\right)$$
$$\sigma^2_{\boldsymbol{\eta}} \sim \mathrm{IG}\left(a, b\right).$$

The hyperparameters $\sigma^2_{\boldsymbol{\beta}}$, $a$ and $b$, as well as the covariance matrix $\boldsymbol{K}$, are fixed constants.

The posterior distribution can be written, up to a constant of proportionality, as

$$\begin{aligned}\pi\left(\boldsymbol{\beta}, \boldsymbol{\eta}, \sigma^2_{\boldsymbol{\eta}} \mid \boldsymbol{Z}\right) \propto \exp&\left\{-\frac{1}{2}\sum_{i=1}^{n} \frac{1}{D_i}\left(Z_i - \boldsymbol{x}_i^\top \boldsymbol{\beta} - \boldsymbol{s}_i^\top \boldsymbol{\eta}\right)^2\right\} \\ &\times \left(\sigma^2_{\boldsymbol{\eta}}\right)^{-r/2} \exp\left\{-\frac{1}{2\sigma^2_{\boldsymbol{\eta}}} \boldsymbol{\eta}^\top \boldsymbol{K}^{-1} \boldsymbol{\eta}\right\} \times \left(\sigma^2_{\boldsymbol{\eta}}\right)^{-a-1} \exp\left\{-\frac{b}{\sigma^2_{\boldsymbol{\eta}}}\right\}.\end{aligned} \tag{B.1}$$

The full conditional distributions of the parameters $\boldsymbol{\beta}$, $\boldsymbol{\eta}$, and $\sigma^2_{\boldsymbol{\eta}}$, for the posterior distribution (B.1) are straight forward to calculate, and are given by

$$\boldsymbol{\beta} \mid \boldsymbol{\eta}, \sigma^2_{\boldsymbol{\eta}}, \boldsymbol{Z} \sim \mathrm{N}_p\left(\boldsymbol{V}_{\boldsymbol{\beta}} \boldsymbol{X}^\top \boldsymbol{D}^{-1}\left(\boldsymbol{Z} - \boldsymbol{S}\boldsymbol{\eta}\right), \boldsymbol{V}_{\boldsymbol{\beta}}\right),$$

where

$$\boldsymbol{V}_{\boldsymbol{\beta}} = \left(\frac{1}{\sigma^2_{\boldsymbol{\beta}}} \boldsymbol{I}_{p\times p} + \boldsymbol{X}^\top \boldsymbol{D}^{-1} \boldsymbol{X}\right)^{-1},$$

$$\boldsymbol{\eta} \mid \boldsymbol{\beta}, \sigma^2_{\boldsymbol{\beta}}, \boldsymbol{Z} \sim \mathrm{N}_r\left(\boldsymbol{V}_{\boldsymbol{\eta}} \boldsymbol{S}^\top \boldsymbol{D}^{-1}\left(\boldsymbol{Z} - \boldsymbol{X}\boldsymbol{\beta}\right), \boldsymbol{V}_{\boldsymbol{\eta}}\right)$$

where

$$\boldsymbol{V}_{\boldsymbol{\eta}} = \left(\frac{1}{\sigma^2_{\boldsymbol{\eta}}} \boldsymbol{K}^{-1} + \boldsymbol{S}^\top \boldsymbol{D}^{-1} \boldsymbol{S}\right)^{-1},$$

and

$$\sigma^2_{\boldsymbol{\eta}} \mid \boldsymbol{\beta}, \boldsymbol{\eta}, \boldsymbol{Z} \sim \mathrm{IG}\left(a + \frac{r}{2}, b + \frac{1}{2} \boldsymbol{\eta}^\top \boldsymbol{K}^{-1} \boldsymbol{\eta}\right).$$

# C Gibbs Sampler for the Multivariate Spatial Mixture Model

In this section, we describe in detail the Gibbs sampler for posterior inference using the multivariate spatial mixture model (MSMM). The data model for the MSMM is given by

$$Z_i = Y_i + \varepsilon_i,$$

where $Z_i$ are the direct survey estimates, $Y_i$ are the true values, and $\varepsilon_i \overset{\text{ind.}}{\sim} \mathrm{N}(0, D_i)$ for known sampling variances $D_i$. The process model is

$$Y_i = \boldsymbol{x}_i^\top \boldsymbol{\beta}_i + \boldsymbol{s}_i^\top \boldsymbol{\eta}_i$$
$$\boldsymbol{\theta}_i^\top = \left(\boldsymbol{\beta}_i^\top, \boldsymbol{\eta}_i^\top\right) \mid G \overset{\text{i.i.d.}}{\sim} G,$$
$$G \sim \mathrm{DP}\left(\alpha, G_0\right),$$

where $\mathrm{DP}\left(\alpha, G_0\right)$ is the Dirichlet process prior with concentration parameter $\alpha$ and base distribution $G_0$. The base distribution, $G_0$, is taken to be a product of independent, mean zero Gaussian distributions, with covariance matrices $\sigma^2_{\boldsymbol{\beta}} \boldsymbol{I}_{p\times p}$ and $\sigma^2_{\boldsymbol{\eta}} \boldsymbol{K}$, corresponding to the $\boldsymbol{\beta}$ and $\boldsymbol{\eta}$ components of $\boldsymbol{\theta}$, respectively. Finally, the parameter model is given by

$$\alpha \sim \mathrm{Gamma}\left(a_\alpha, b_\alpha\right)$$
$$\sigma^2_{\boldsymbol{\eta}} \sim \mathrm{IG}\left(a_{\boldsymbol{\eta}}, b_{\boldsymbol{\eta}}\right),$$

for fixed hyperparameters $a_\alpha, b_\alpha, a_{\boldsymbol{\eta}}, b_{\boldsymbol{\eta}}$, and $\sigma^2_{\boldsymbol{\beta}}$.

Let $c_i$ be the latent class variables defining the cluster membership for the observations $Z_i$. For each distinct class $c$, let $\boldsymbol{\theta}_c$ be the parameters corresponding to that class. To draw samples from the posterior distribution

$$\pi\left(\boldsymbol{\theta}, \boldsymbol{c}, \alpha, \sigma_{\boldsymbol{\eta}}^2 \mid \boldsymbol{Z}\right),$$

we use Gibbs sampling, following Algorithm 2 in Neal (2000).

The marginal distribution of $Z_i$, and the posterior distribution of $\boldsymbol{\theta}$, based on the prior $g_0(\boldsymbol{\theta})$, are needed to derive the full conditional distributions for the unknown parameters. Let $\boldsymbol{\xi}_i^\top = \left(\boldsymbol{x}_i^\top, \boldsymbol{s}_i^\top\right)$, $\boldsymbol{D}$ be a diagonal matrix of the sampling variances $D_i$, and $\boldsymbol{\Sigma}$ be a block-diagonal matrix consisting of the covariances $\sigma_\beta^2 \boldsymbol{I}_{p\times p}$ and $\sigma_\eta^2 \boldsymbol{K}$. Use of the Sherman-Morrison formula and straightforward calculations, gives

$$Z_i \sim N\left(0, D_i + \boldsymbol{\xi}_i^\top \boldsymbol{\Sigma} \boldsymbol{\xi}_i\right) \tag{C.1}$$

and

$$\boldsymbol{\theta} \mid Z_i \sim \mathrm{N}_{p+r}\left(\left(\frac{1}{D_i}\boldsymbol{\xi}\boldsymbol{\xi}_i^\top + \boldsymbol{\Sigma}^{-1}\right)^{-1} \boldsymbol{\xi}_i \frac{Z_i}{D_i}, \left(\frac{1}{D_i}\boldsymbol{\xi}_i\boldsymbol{\xi}_i^\top + \boldsymbol{\Sigma}^{-1}\right)^{-1}\right). \tag{C.2}$$

Suppose we have sampled values $\alpha^{(t-1)}$, $\boldsymbol{\theta}^{(t-1)}$, $\boldsymbol{c}^{(t-1)}$, and $\sigma_{\boldsymbol{\eta}}^{2(t-1)}$ from the $(t-1)$st iteration of the Gibbs sampler. The parameters can be updated at the $t$th iteration of the Gibbs sampler using the full conditional distributions of the parameters, given the parameter values at the $(t-1)$st iteration.

West (1992) showed that the full conditional distribution for $\alpha$ depends only on the number of unique clusters $c^*$, and used a data augmentation technique for sampling from the full conditional distribution. Given $\alpha^{(t-1)}$ and $c^{*(t-1)}$, draw $x$ from a Beta$(\alpha^{(t-1)}+1, n)$ distribution. Define a weight, $\pi_x$, by

$$\frac{\pi_x}{1-\pi_x} = \frac{a_\alpha + c^{*(t-1)} - 1}{n\left(b_\alpha - \log(x)\right)}.$$

Then, $\alpha$ is updated with a draw from the mixture distribution

$$\alpha^{(t)} \sim \pi_x \mathrm{Gamma}\left(a_\alpha + c^{*(t-1)}, b_\alpha - \log(x)\right) + (1-\pi_x)\mathrm{Gamma}\left(a_\alpha + c^{*(t-1)} - 1, b_\alpha - \log(x)\right).$$

For updating the class labels, $c_i$, define $\boldsymbol{c}_{-i}$ to be the current state of the class labels $\boldsymbol{c}$, with the value $c_i$ removed. Let $\mathcal{C}$ be the collection of unique values in $\boldsymbol{c}_{-i}$ and let $n_{-i,c}$ be the number of $c_j \in \boldsymbol{c}_{-i}$ such that $c_j = c$ for each $c \in \mathcal{C}$. Following Algorithm 2 of Neal (2000),

$$\begin{aligned} P\left(c_i^{(t)} = c \mid \boldsymbol{c}_{-i}, \boldsymbol{\theta}^{(t-1)}, \sigma_\eta^{2(t-1)}, \alpha^{(t)}, \boldsymbol{Z}\right) &\propto \frac{n_{-i,c}}{n-1+\alpha^{(t)}} f\left(Z_i \mid \boldsymbol{\theta}_c\right) \\ P\left(c_i^{(t)} \neq c_j \text{ for all } c_j \in \boldsymbol{c}_{-i} \mid \boldsymbol{c}_{-i}, \boldsymbol{\theta}^{(t-1)}, \sigma_\eta^{2(t-1)}, \alpha^{(t-1)}, \boldsymbol{Z}\right) &\propto \frac{\alpha}{n-i+\alpha} f(Z_i), \end{aligned} \tag{C.3}$$

where $f(Z_i)$ is the marginal distribution in (C.1).

It is possible that a non-empty cluster at the $(t-1)$st iteration becomes empty at the $t$th iteration of the Gibbs sampler. In this situation, this cluster can simply be removed from the MCMC chain. Also, the second line of (C.3) implies that a new cluster, with one element $i$, can be created at any iteration. In this situation, parameters $\boldsymbol{\theta}_c$ are drawn from the posterior distribution (C.2), and added to the current state of the MCMC chain.

The full conditional distributions for the remaining parameters, $\boldsymbol{\theta}$ and $\sigma_{\boldsymbol{\eta}}^2$, belong to standard parametric families. For each $c \in \mathcal{C}$,

$$\boldsymbol{\theta}_c^{(t)} \mid \boldsymbol{c}^{(t)}, \sigma_\eta^{2(t-1)}, \boldsymbol{\alpha}^{(t)}, \boldsymbol{Z} \sim \mathrm{N}_{p+r}\left(\boldsymbol{\mu}_\theta, \boldsymbol{V}_\theta\right),$$

where

$$\boldsymbol{V}_\theta = \left(\boldsymbol{\Sigma}^{-1} + \boldsymbol{\xi}_c^\top \boldsymbol{D}_c^{-1} \boldsymbol{\xi}_c\right)^{-1}$$

and

$$\boldsymbol{\mu}_\theta = \boldsymbol{V}_\theta \boldsymbol{\xi}_c^\top \boldsymbol{D}_c^{-1} \boldsymbol{Z}_c.$$

Here, $\boldsymbol{\xi}_c$, $\boldsymbol{D}_c$, and $\boldsymbol{Z}_c$ are the subsets of the matrices $\boldsymbol{\xi}$, $\boldsymbol{D}$, and $\boldsymbol{Z}$ corresponding to the elements $i$ such that $c_i^{(t)} = c$.

Finally, the full conditional distribution for the variance component $\sigma_\eta^2$ belongs to the Inverse Gamma family:

$$\sigma_\eta^{2(t)} \mid \boldsymbol{\theta}^{(t)}, \boldsymbol{c}^{(t)}, \alpha^{(t)}, \sim \text{IG}\left(a_\eta + rc^{*(t)}/2, b_\eta + 0.5 \sum_{c \in \mathcal{C}} \boldsymbol{\eta}_c^\top \boldsymbol{K}^{-1} \boldsymbol{\eta}_c\right).$$

# D Stick-Breaking Multivariate Spatial Mixture Model

This section describes a stick-breaking version of the Dirichlet process mixture discussed in Section C, including a Gibbs sampler which can produce draws from its posterior distribution. Here, the data model is

$$Z_i = Y_i + \epsilon_i, \quad \epsilon_i \overset{\text{ind.}}{\sim} \text{N}(0, D_i),$$

for $i = 1, \dots, n$. The process model is

$$\begin{aligned} &Y_i = \boldsymbol{x}_i^\top \boldsymbol{\beta}_{W_i} + \boldsymbol{s}_i^\top \boldsymbol{\eta}_{W_i}, \\ &W_i \sim \text{Discrete}(1, \dots, J; \boldsymbol{\pi}), \quad \boldsymbol{\pi} = \text{stick}(\phi_1, \dots, \phi_{J-1}), \\ &\phi_j \sim \text{Beta}(1, \alpha), \end{aligned}$$

for $j = 1, \dots, J$ using the function

$$\text{stick}(\boldsymbol{\phi}) = \left(\phi_1 \prod_{\ell=1}^{0}(1-\phi_\ell),\ \phi_2 \prod_{\ell=1}^{1}(1-\phi_\ell),\ \dots,\ \phi_J \prod_{\ell=1}^{J-1}(1-\phi_\ell)\right),$$

where $\phi_J \equiv 1$. The notation $\text{Discrete}(1, \dots, J; \boldsymbol{\pi})$ represents a discrete distribution with values $(1, \dots, J)$ having respective probabilities $\boldsymbol{\pi} = (\pi_1, \dots, \pi_J)$. The parameter model is

$$\boldsymbol{\beta}_j \sim \text{N}(\boldsymbol{0}, \sigma_\beta^2 \boldsymbol{I}_p), \quad \boldsymbol{\eta}_j \sim \text{N}\left(\boldsymbol{0}, \sigma_j^2 \boldsymbol{K}\right), \quad \sigma_j^2 \sim \text{IG}(\alpha_K, \beta_K), \quad \alpha \sim \text{Gamma}(a_\alpha, b_\alpha).$$

Here, $J$ represents the maximum number of clusters in the data, and must be specified by the analyst. Clusters here have been specified at the observation level, so that any distinct $i, i' \in \{1, \dots, n\}$ may be assigned to different clusters, whether they share common geography or contingency table factors. Hyperparameters in this model are $\sigma_\beta^2$, $\alpha_\xi$, $\beta_\xi$, $\alpha_K$, and $\beta_K$.

Denote $\text{N}(x \mid \mu, \sigma^2)$, $\text{IG}(x \mid a, b) \propto x^{-a-1} e^{-b/x} I(x > 0)$, $\text{Gamma}(x \mid a, b) \propto x^{a-1} e^{-bx} I(x > 0)$, and $\text{Beta}(x \mid a, b)$ as the density functions of distributions $\text{N}(\mu, \sigma^2)$, $\text{IG}(a, b)$, $\text{Gamma}(a, b)$, and $\text{Beta}(a, b)$, respectively. From the model specification, the joint distribution of all random quantities is

$$\begin{aligned} f(\boldsymbol{Z}, \boldsymbol{W}, \boldsymbol{\phi}, \boldsymbol{\beta}, \boldsymbol{\eta}, \boldsymbol{\sigma}^2, \alpha) = &\prod_{i=1}^{n} \prod_{j=1}^{J} \left[\pi_j \text{N}(Z_i \mid \boldsymbol{x}_i^\top \boldsymbol{\beta}_j + \boldsymbol{s}_i^\top \boldsymbol{\eta}_j, D_i)\right]^{I(w_i = j)} \prod_{j=1}^{J} \text{N}(\boldsymbol{\eta}_j \mid \boldsymbol{0}, \sigma_j^2 \boldsymbol{K}) \\ &\times \prod_{j=1}^{J} \text{N}(\boldsymbol{\beta}_j \mid \boldsymbol{0}, \sigma_\beta^2 \boldsymbol{I}) \prod_{j=1}^{J} \text{IG}(\sigma_j^2 \mid a_K, b_K) \prod_{j=1}^{J-1} \text{Beta}(\phi \mid 1, \alpha) \\ &\times \text{Gamma}(\alpha \mid a_\alpha, b_\alpha). \end{aligned} \tag{D.1}$$

The full conditionals of (D.1) yield the Gibbs sampler. Because the calculations are straightforward, only the final expressions are given. Let $[X \mid \cdots]$ denote the distribution of random variable $X$ conditional on all other random quantities in the model. Let $\boldsymbol{Z}_j = \text{Vec}(Z_i : W_i = j)$, $\boldsymbol{D}_j = \text{Diag}(D_i : W_i = j)$. Let $\boldsymbol{X}_j$ and $\boldsymbol{S}_j$ denote matrices composed of rows $\boldsymbol{x}_i^\top$ and $\boldsymbol{s}_i^\top$, respectively, for $\{i : W_i = j\}$. We have

1. $[\phi_1, \dots, \phi_{J-1} \mid \cdots] = \prod_{j=1}^{J-1} \text{Beta}\left(\phi_j \mid 1 + n_j, \alpha + \sum_{b=j+1}^{J} n_b\right)$ where $n_j = \sum_{i=1}^{n} I(w_i = j)$.

2. $[\alpha \mid \cdots] = \text{Gamma}\left(\alpha \mid a_\alpha, b_\alpha - \sum_{j=1}^{J-1} \log(1-\phi_j)\right)$.

3. $[\boldsymbol{\eta}_1, \ldots, \boldsymbol{\eta}_J \mid \cdots] = \prod_{j=1}^J \text{N}(\boldsymbol{\eta}_j \mid \boldsymbol{\vartheta}_j, \boldsymbol{\Omega}_j^{-1})$ with $\boldsymbol{\Omega}_j = \sigma_j^{-2}\boldsymbol{K}^{-1} + \boldsymbol{S}_j\boldsymbol{D}_j^{-1}\boldsymbol{S}_j$, and $\boldsymbol{\vartheta}_j = \boldsymbol{\Omega}_j^{-1}\boldsymbol{S}_j^\top \boldsymbol{D}_j^{-1}(\boldsymbol{Z}_j - \boldsymbol{X}_j\boldsymbol{\beta}_j)$.

4. $[\boldsymbol{\beta}_1, \ldots, \boldsymbol{\beta}_J \mid \cdots] = \prod_{j=1}^J \text{N}(\boldsymbol{\beta}_j \mid \boldsymbol{\vartheta}_j, \boldsymbol{\Omega}_j^{-1})$ with $\boldsymbol{\Omega}_j = \sigma_\beta^{-2}\boldsymbol{I} + \boldsymbol{X}_j\boldsymbol{D}_j^{-1}\boldsymbol{X}_j$, and $\boldsymbol{\vartheta}_j = \boldsymbol{\Omega}_j^{-1}\boldsymbol{X}_j^\top \boldsymbol{D}_j^{-1}(\boldsymbol{Z}_j - \boldsymbol{S}_j\boldsymbol{\eta}_j)$.

5. $[\sigma_1^2, \ldots, \sigma_J^2 \mid \cdots] = \prod_{j=1}^J \text{IG}\left(\sigma_j^2 \mid a_K + \frac{1}{2}r, b_K + \frac{1}{2}\boldsymbol{\eta}_j^\top \boldsymbol{K}^{-1}\boldsymbol{\eta}_j\right)$.

6. $[W_1, \ldots, W_n \mid \cdots] = \prod_{i=1}^n \text{Discrete}(W_i \mid \tilde{\pi}_{i1}, \ldots, \tilde{\pi}_{iJ})$, where $\tilde{\pi}_{ij} = \frac{\pi_j \text{N}(Z_i \mid \boldsymbol{x}_i^\top \boldsymbol{\beta}_j + \boldsymbol{s}_i^\top \boldsymbol{\eta}_j, D_i)}{\sum_{\ell=1}^J \pi_\ell \text{N}(Z_i \mid \boldsymbol{x}_i^\top \boldsymbol{\beta}_\ell + \boldsymbol{s}_i^\top \boldsymbol{\eta}_\ell, D_i)}$ for $j = 1, \ldots, J$.

To see that the stick-breaking model produces similar results to the DP model in Section C, Figure 1 compares estimates of $\text{E}(\boldsymbol{Y} \mid \boldsymbol{Z})$ from 4 of the 100 repetitions used in the simulation study in Section 5 of the main article.

# E Computation of Basis Functions

The MSM and MSMM variants feature design vectors $\boldsymbol{s}_i^\top = (s_{i1}, \ldots, s_{ir})$, for $i = 1, \ldots, n$ and $i = 1, \ldots, r$, to be computed from proposed multivariate spatial basis functions. Recall that the matrix $\boldsymbol{S} = (\boldsymbol{s}_1^\top \cdots \boldsymbol{s}_n^\top)^\top$ is obtained from the eigenvectors of $\boldsymbol{G} = (\boldsymbol{I}_n - \boldsymbol{P}_X)\boldsymbol{A}(\boldsymbol{I}_n - \boldsymbol{P}_X)$, where $\boldsymbol{P}_X = \boldsymbol{X}(\boldsymbol{X}^\top\boldsymbol{X})^{-1}\boldsymbol{X}^\top$ and $\boldsymbol{A} = \boldsymbol{W} \otimes \boldsymbol{1}_L\boldsymbol{1}_L^\top$ is the multivariate adjacency matrix. With $\boldsymbol{S}$ in hand, a precision matrix $\boldsymbol{K}^{-1}$ is then specified to induce multivariate and spatial dependencies in the process model. Matrices $\boldsymbol{S}$ and $\boldsymbol{K}^{-1}$ need to be computed only once, prior to implementation of the Gibbs sampler. Naïve computation of $\boldsymbol{S}$ may involve operating on very large dense matrices; however, our particular regression model yields simplifications which are discussed in this section. For the remainder of this section, we will make use of the Kronecker product notation

$$\boldsymbol{A} \otimes \boldsymbol{B} = \begin{pmatrix} a_{11}\boldsymbol{B} & \cdots & a_{1n}\boldsymbol{B} \\ \vdots & & \vdots \\ a_{m1}\boldsymbol{B} & \cdots & a_{mn}\boldsymbol{B} \end{pmatrix}.$$

where $\boldsymbol{A} = (a_{ij}) \in \mathbb{R}^{m \times n}$ and $\boldsymbol{B} \in \mathbb{R}^{p \times q}$.

For the $\boldsymbol{X\beta}$ portion of our models, we have assumed the form

$$\boldsymbol{x}_i^\top \boldsymbol{\beta} = \beta_{0,\ell_i} + t_i\beta_1$$

where $\ell_i$ indexes the contingency table cell for the $i$th observation, and $t_i$ represents the logarithm of one plus the population count for its county. We will assume that $\boldsymbol{t} = (t_1, \ldots, t_m)$ have been centered and scaled. Because all table cells are observed in all counties, we may write

$$\boldsymbol{X} = \begin{pmatrix} \boldsymbol{I}_L & t_1\boldsymbol{1}_L \\ \vdots & \vdots \\ \boldsymbol{I}_L & t_m\boldsymbol{1}_L \end{pmatrix},$$

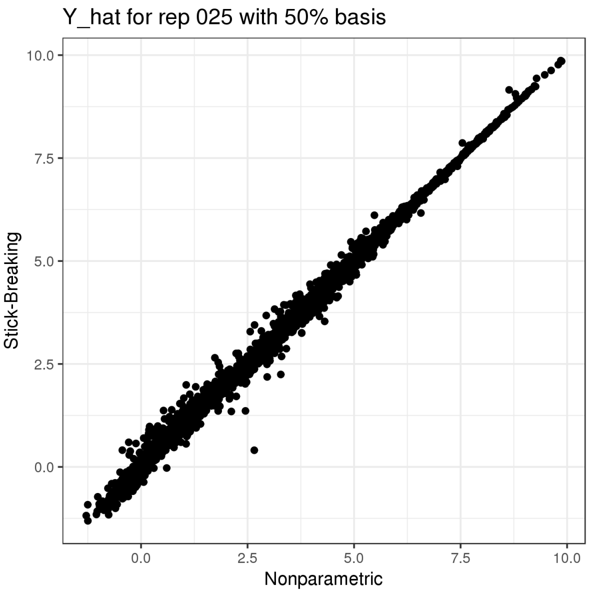


(a)

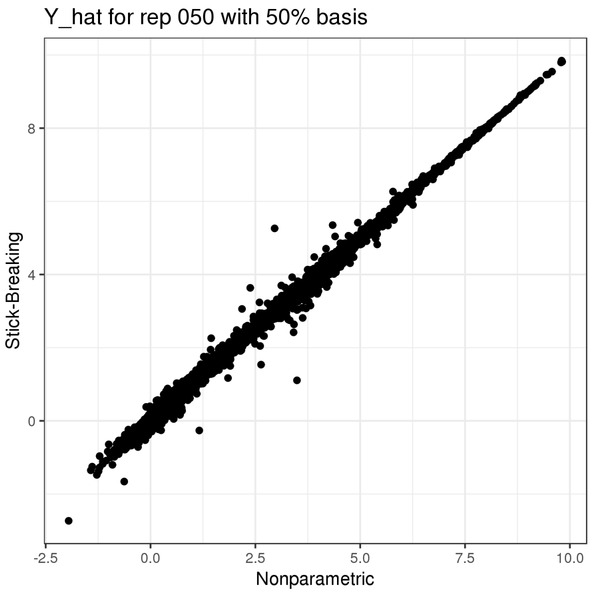


(b)

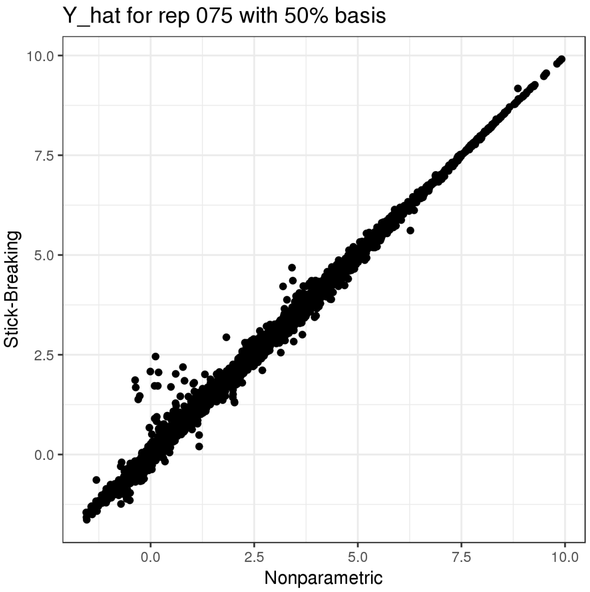


(c)

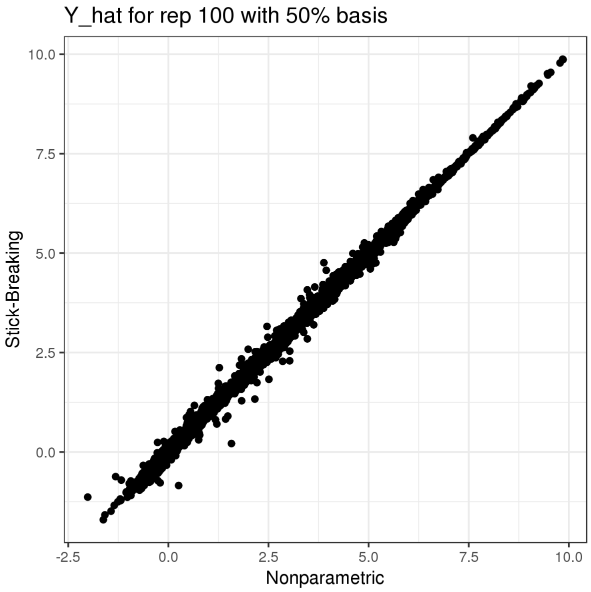


(d)

Figure 1: Comparison between estimates stick breaking model from Section D and DP model from Section C from four simulated datasets. These datasets were produced in repetitions 25, 50, 75, and 100 of the simulation study in Section 5 of the main article. Estimates are displayed on the log-scale in which they have been fitted.

so that

$$
\begin{aligned}
\boldsymbol{P}_X &= \boldsymbol{X}(\boldsymbol{X}^\top \boldsymbol{X})^{-1}\boldsymbol{X}^\top \\
&= \begin{pmatrix} \boldsymbol{I}_L & t_1 \mathbf{1}_L \\ \vdots & \vdots \\ \boldsymbol{I}_L & t_m \mathbf{1}_L \end{pmatrix} \begin{pmatrix} m^{-1}\boldsymbol{I}_L & \mathbf{0} \\ \mathbf{0} & n^{-1} \end{pmatrix} \begin{pmatrix} \boldsymbol{I}_L & \cdots & \boldsymbol{I}_L \\ t_1 \mathbf{1}_L & \cdots & t_m \mathbf{1}_L \end{pmatrix} \\
&= \begin{pmatrix} m^{-1}\boldsymbol{I}_L + n^{-1} t_1 t_1 \mathbf{1}_L \mathbf{1}_L^\top & \cdots & m^{-1}\boldsymbol{I}_L + n^{-1} t_1 t_m \mathbf{1}_L \mathbf{1}_L^\top \\ \vdots & & \vdots \\ m^{-1}\boldsymbol{I}_L + n^{-1} t_m t_1 \mathbf{1}_L \mathbf{1}_L^\top & \cdots & m^{-1}\boldsymbol{I}_L + n^{-1} t_m t_m \mathbf{1}_L \mathbf{1}_L^\top \end{pmatrix} \\
&= (\mathbf{1}_m \mathbf{1}_m^\top \otimes m^{-1}\boldsymbol{I}_L) + (n^{-1}\boldsymbol{t}\boldsymbol{t}^\top \otimes \mathbf{1}_L \mathbf{1}_L^\top).
\end{aligned}
$$

Using

$$
\begin{aligned}
\boldsymbol{P}_X \boldsymbol{A} &= (\mathbf{1}_m \mathbf{1}_m^\top \otimes m^{-1}\boldsymbol{I}_L)[\boldsymbol{W} \otimes \mathbf{1}_L \mathbf{1}_L^\top] + (n^{-1}\boldsymbol{t}\boldsymbol{t}^\top \otimes \mathbf{1}_L \mathbf{1}_L^\top)[\boldsymbol{W} \otimes \mathbf{1}_L \mathbf{1}_L^\top] \\
&= (m^{-1}\mathbf{1}_m \mathbf{1}_m^\top \boldsymbol{W} + m^{-1}\boldsymbol{t}\boldsymbol{t}^\top \boldsymbol{W}) \otimes \mathbf{1}_L \mathbf{1}_L^\top
\end{aligned}
$$

and

$$
\begin{aligned}
\boldsymbol{P}_X \boldsymbol{A} \boldsymbol{P}_X &= [(m^{-1}\mathbf{1}_m \mathbf{1}_m^\top \boldsymbol{W} + m^{-1}\boldsymbol{t}\boldsymbol{t}^\top \boldsymbol{W}) \otimes \mathbf{1}_L \mathbf{1}_L^\top][(\mathbf{1}_m \mathbf{1}_m^\top \otimes m^{-1}\boldsymbol{I}_L) + (n^{-1}\boldsymbol{t}\boldsymbol{t}^\top \otimes \mathbf{1}_L \mathbf{1}_L^\top)] \\
&= [m^{-2}\mathbf{1}_m \mathbf{1}_m^\top \boldsymbol{W} \mathbf{1}_m \mathbf{1}_m^\top + m^{-2}\boldsymbol{t}\boldsymbol{t}^\top \boldsymbol{W} \mathbf{1}_m \mathbf{1}_m^\top + m^{-2}\mathbf{1}_m \mathbf{1}_m^\top \boldsymbol{W} \boldsymbol{t}\boldsymbol{t}^\top + m^{-2}\boldsymbol{t}\boldsymbol{t}^\top \boldsymbol{W} \boldsymbol{t}\boldsymbol{t}^\top] \otimes \mathbf{1}_L \mathbf{1}_L^\top
\end{aligned}
$$

we have

$$
\begin{aligned}
\boldsymbol{G} &= (\boldsymbol{I} - \boldsymbol{P}_X)\boldsymbol{A}(\boldsymbol{I} - \boldsymbol{P}_X) \\
&= \boldsymbol{A} - \boldsymbol{P}_X \boldsymbol{A} - (\boldsymbol{P}_X \boldsymbol{A})^\top + \boldsymbol{P}_X \boldsymbol{A} \boldsymbol{P}_X \\
&= \tilde{\boldsymbol{G}} \otimes \mathbf{1}_L \mathbf{1}_L^\top, \qquad \text{(E.1)}
\end{aligned}
$$

where

$$
\begin{aligned}
\tilde{\boldsymbol{G}} = \boldsymbol{W} &- m^{-1}\mathbf{1}_m \mathbf{1}_m^\top \boldsymbol{W} - m^{-1}\boldsymbol{t}\boldsymbol{t}^\top \boldsymbol{W} - m^{-1}\boldsymbol{W}^\top \mathbf{1}_m \mathbf{1}_m^\top - m^{-1}\boldsymbol{W}^\top \boldsymbol{t}\boldsymbol{t}^\top \\
&+ m^{-2}\mathbf{1}_m \mathbf{1}_m^\top \boldsymbol{W} \mathbf{1}_m \mathbf{1}_m^\top + m^{-2}\boldsymbol{t}\boldsymbol{t}^\top \boldsymbol{W} \mathbf{1}_m \mathbf{1}_m^\top + m^{-2}\mathbf{1}_m \mathbf{1}_m^\top \boldsymbol{W} \boldsymbol{t}\boldsymbol{t}^\top + m^{-2}\boldsymbol{t}\boldsymbol{t}^\top \boldsymbol{W} \boldsymbol{t}\boldsymbol{t}^\top.
\end{aligned}
$$

Now, to compute eigenvectors of (E.1), let $\tilde{\boldsymbol{G}} = \boldsymbol{U}\,\mathrm{Diag}(\boldsymbol{\lambda})\boldsymbol{U}^\top$ so that $\boldsymbol{\lambda} = (\lambda_1, \ldots, \lambda_m)$ are eigenvalues and columns of $\boldsymbol{U} = (\boldsymbol{u}_1, \ldots, \boldsymbol{u}_m)$ are corresponding eigenvectors. A similar decomposition for $\mathbf{1}_L \mathbf{1}_L^\top = \boldsymbol{V}\,\mathrm{Diag}(\boldsymbol{\mu})\boldsymbol{V}^\top$ gives $\mu_1 = L$ with corresponding eigenvector $\boldsymbol{v}_1 = \mathbf{1}_L/\sqrt{L}$, and $\mu_2 = \cdots = \mu_L = 0$ corresponding to eigenvectors $\boldsymbol{v}_2, \ldots, \boldsymbol{v}_L$. For any $\boldsymbol{u}_i$ and $\boldsymbol{v}_j$,

$$
\boldsymbol{G}(\boldsymbol{u}_i \otimes \boldsymbol{v}_j) = [\tilde{\boldsymbol{G}} \otimes \mathbf{1}_L \mathbf{1}_L^\top](\boldsymbol{u}_i \otimes \boldsymbol{v}_j) = (\tilde{\boldsymbol{G}}\boldsymbol{u}_i) \otimes (\mathbf{1}_L \mathbf{1}_L^\top \boldsymbol{v}_j) = (\lambda_i \boldsymbol{u}_i) \otimes (\mu_j \boldsymbol{v}_j) = \lambda_i \mu_j (\boldsymbol{u}_i \otimes \boldsymbol{v}_j),
$$

so that $\boldsymbol{u}_i \otimes \boldsymbol{v}_j$ is an eigenvector of $\boldsymbol{G}$ with corresponding eigenvalue $\lambda_i \mu_j$. The eigenvectors of $\boldsymbol{G}$ are therefore the columns of

$$
\boldsymbol{U} \otimes \boldsymbol{V} = \left( \begin{array}{ccc|c|ccc} \boldsymbol{u}_1 \otimes \boldsymbol{v}_1 & \cdots & \boldsymbol{u}_1 \otimes \boldsymbol{v}_L & \cdots & \boldsymbol{u}_m \otimes \boldsymbol{v}_1 & \cdots & \boldsymbol{u}_m \otimes \boldsymbol{v}_L \end{array} \right),
$$

and the corresponding eigenvalues are the entries of $\boldsymbol{\lambda} \otimes \boldsymbol{\mu}$.

# F Design of the empirical simulation study

The dataset analyzed in Section 3.2, and used for the empirical simulation study of Section 5 of the main paper, consists of American Community Survey (ACS) 5-year estimates of the counts of children, ages 0–1,

2–3, and 4–5, in each of seven race categories, White alone, Black alone, Asian alone, American Indian or Alaska Native alone, Native Hawaiian or Pacific Islander alone, Other alone, or two or more races, in counties in Minnesota and the surrounding states. In addition, design-based estimates of the variances of the ACS counts are included in the data set. Both the direct estimates, $Z_i^*$, and the design-based estimates of their variances, $D_i^*$, are part of this publicly available dataset.

In the main paper, we fit the MSMM to the log-transformed direct estimates, $Z_i = \log(Z_i^* + 1)$, which can be obtained from the publicly available data. However, variance estimates of the $Z_i$ require access to a set of replicate weights, which are not publicly available. In order to provide an example in the main paper which can be replicated, we use a set of variance estimates, $D_i$, which use the Delta method and some smoothing, and can be constructed from the $Z_i^*$ and the $D_i^*$ as follows: first, the Delta method is used to obtain rough estimates of the variances of the $Z_i^*$,

$$\tilde{D}_i = \frac{D_i^*}{Z_i^* + 1}.$$

Because many of the $Z_i$ are small or equal to zero, the $\tilde{D}_i$ are not stable for areas with small sample size. However, the $\tilde{D}_i$ appear to agree quite closely to the variance estimates constructed using replicate weights for areas with moderate and large sample size. To smooth the $\tilde{D}_i$ to more closely resemble the variances constructed using replicate weights, we define $D_i = \tilde{D}_i$ if $\tilde{D}_i \leq 1.5$, $D_i = 0.637 + 0.055\tilde{D}_i$ if $1.5 < \tilde{D}_i \leq 4$, and $D_i = \tilde{D}_i/10$ if $\tilde{D}_i > 4$. In the empirical simulation study of Section 5, we used these $D_i$ as the 'true' sampling variances in the model. In the data analysis done in Section 3.2, we used the variance estimates constructed using replicate weights, which are not publicly available, as model inputs.


## Acknowledgements

The DRB approval number for this paper is CDBRB-FY20-044. This report is released to inform interested parties of ongoing research and to encourage discussion of work in progress. The views expressed are those of the authors, and not those of the U.S. Census Bureau.


# References


Neal, R. M. (2000). Markov chain sampling methods for Dirichlet process mixture models. *Journal of Computational and Graphical Statistics*, 9(2):249 – 265.

West, M. (1992). Hyperparameter estimation in Dirichlet process mixture models. Technical report, Institute of Statistics and Decision Sciences, Duke University.
